# Supplementary material for: Delayed dynamic triggering and enhanced high-frequency seismic radiation due to brittle rock damage in 3D multi-fault rupture simulations
Source: arXiv:2503.21260 source file (2025-03-27)
Supplement: Supplementary file 1 [file SI.pdf]

# Supporting Information for "Delayed dynamic triggering and enhanced high-frequency seismic radiation due to brittle rock damage in 3D multi-fault rupture simulations"

Zihua Niu[1], Alice-Agnes Gabriel[2,1], Yehuda Ben-Zion[3,4]

[1]Department of Earth and Environmental Sciences, Ludwig-Maximilians-Universität München, Munich, Germany

[2]Scripps Institution of Oceanography, UC San Diego, La Jolla, CA, USA

[3]Department of Earth Sciences, University of Southern California, Los Angeles, CA, USA

[4]Statewide California Earthquake Center, University of Southern California, Los Angeles, CA, USA

## Contents of this file

1. Text S1 to S7

2. Figures S1 to S6

3. Tables S1 to S2

## Additional Supporting Information (Files uploaded separately)

1. Captions for Movies S1 to S4

## Introduction

The results we present in this work are based on a new discontinuous Galerkin algorithm that we develop and apply to combine dynamic rupture simulation with wave propagation utilizing the continuum damage breakage damage (CDB) model (Lyakhovsky & Ben-Zion, 2014; Lyakhovsky et al., 2016) in 3D. This supplementary file includes detailed information on the methods and model configurations. We show verifications of our algorithm and implementation with (1) off-fault damage pattern and (2) high-frequency seismic radiations using meshes with different resolutions. Additional results that support the effects of 3D co-seismic off-fault damage on the rupture dynamics and earthquake interaction are also provided here. They include (1) damage-dependent supershear transition, (2) damage-dependent size of the cohesive zone, and (3) time-dependent distributions of slip rate, fault slip and shear traction on the two faults in the TPV23 setup shown in the main text.

## Text S1: Continuum damage breakage model and its implementation in SeisSol for 3D dynamic rupture modeling

In the following, we summarize the governing equations of the CDB model. To demonstrate how it fits into the numerical algorithms proposed by Niu et al. (2025) for SeisSol, we formulate the governing equations into nonlinear hyperbolic partial differential equations. We can adapt the same prediction-correction time stepping and the numerical fluxes for free-surface and absorbing boundaries. However, in this section, we need to further specify how we deal with the friction boundary for dynamic rupture simulations. This procedure essentially involves: (1) a derivation of the traction on both sides of the fault in the fault-aligned coordinate system and (2) a derivation of the effective moduli that account for the accumulation of off-fault damage.

The CDB model is proposed within the framework of continuum mechanics. The mechanical response of rocks from their intact states to their failure is mathematically described by a scalar damage variable ($\alpha$) that represents the density of distributed microcracks and a scalar breakage variable ($B$) describing the grain size distribution in the post-failure stage of rocks (Einav, 2007b,a). In CDB, the latter stage is named the granular phase (Lyakhovsky et al., 2016). Both $\alpha$ and $B$ are defined in the range of [0,1]. In analogy to Niu et al. (2025), the governing equations of the CDB model are

$$\begin{cases} \dfrac{\partial \varepsilon_{ij}}{\partial t} & = \dfrac{1}{2}(\dfrac{\partial v_i}{\partial x_j} + \dfrac{\partial v_j}{\partial x_i}) \\ \rho \dfrac{\partial v_i}{\partial t} & = \dfrac{\partial \sigma_{ij}(\underline{\underline{\varepsilon}}, \alpha, B)}{\partial x_j} \\ \dfrac{\partial \alpha}{\partial t} & = r_\alpha(\underline{\underline{\varepsilon}}, \alpha, B) \\ \dfrac{\partial B}{\partial t} & = r_B(\underline{\underline{\varepsilon}}, \alpha, B) \end{cases}, \tag{1}$$

where $\underset{=}{\varepsilon} = \varepsilon_{ij}$ and $\sigma_{ij}$ denote strain and stress tensor, $v_i$ is the vector for particle velocity, and $\rho$ is material mass density. $\alpha$ is a damage variable and $B$ is a breakage variable. $r_\alpha$ and $r_B$ are two functions of the strain tensor, the damage variable and the breakage variable. We provide the expressions for $\sigma_{ij}$, $r_\alpha$ and $r_B$ in the CDB model as follows:

$$\begin{cases} \sigma_{ij}(\underset{=}{\varepsilon}, \alpha, B) = (1-B)\sigma_{ij}^s + B\sigma_{ij}^b \\ r_\alpha(\underset{=}{\varepsilon}, \alpha, B) = \begin{cases} C_d(1-B)\gamma_r I_2(\xi - \xi_0) & \text{, if } \xi - \xi_0 > 0 \\ 0 & \text{, if } \xi - \xi_0 \leq 0 \end{cases} \\ r_B(\underset{=}{\varepsilon}, \alpha, B) = \begin{cases} C_B(1-B)P(\alpha)\gamma_r I_2(\xi - \xi_0) & \text{, if } \xi - \xi_0 > 0 \\ 0 & \text{, if } \xi - \xi_0 \leq 0 \end{cases} \end{cases}, \quad (2)$$

where $\sigma_{ij}^s = \lambda_0 I_1 \delta_{ij} - \alpha\gamma_r\sqrt{I_2}\delta_{ij} + [2(\mu_0 + \alpha\gamma_r\xi_0) - \alpha\gamma_r\xi]\varepsilon_{ij}$ is the stress-strain relationship for solid state of the material. $\gamma_r$ is the nonlinear modulus. $I_1 = \varepsilon_{kk}$ and $I_2 = \varepsilon_{ij}\varepsilon_{ij}$ are the first and the second strain invariant. $\xi = I_1/\sqrt{I_2}$ is derived from the two strain invariants. It grows from $-\sqrt{3}$ for isotropic compression to $\sqrt{3}$ for isotropic extension. The damage $\alpha$ starts to accumulate as the strain state deviates farther enough from the isotropic compression. This is formulated as $\xi - \xi_0 > 0$, where $\xi_0$ is the strain invariants ratio that defines the onset of damage accumulation. This is usually negative for rocks (Lyakhovsky et al., 2016), suggesting the damage can also accumulate when the isotropic component of the stress tensor $I_1$ remains negative, i.e., when the material is under compression. $C_d$ is a constant damage evolution coefficient that governs the rate of damage accumulation. When the value of $\alpha$ accumulates beyond its critical value $\alpha_{cr}(\xi)$, the solid phase becomes mechanically unstable (Lyakhovsky & Ben-Zion, 2014) and transits into granular phase.

$\sigma_{ij}^b = (2a_2 + 3a_3\xi)I_1\delta_{ij} + a_1\sqrt{I_2}\delta_{ij} + (2a_0 + a_1\xi - a_3\xi^3)\varepsilon_{ij}$ is the stress-strain relationship for granular phase of the material (Lyakhovsky et al., 2016). The granular phase moduli

from $a_0$ to $a_3$ ensure the mechanical stability of the material during the transition from the solid phase to the granular phase (Lyakhovsky & Ben-Zion, 2014).

$C_B$ is the breakage evolution coefficient that governs the rate of breakage accumulation. It is further scaled by $P(\alpha) = \dfrac{1}{\exp\left(\dfrac{\alpha_{cr} - \alpha}{\beta}\right) + 1}$, which is the probability of the material to be in the granular phase (Lyakhovsky & Ben-Zion, 2014). The breakage accumulation rate becomes significant when $\alpha \to \alpha_{cr}$. This represents the rapid transition from the solid ($B = 0$) to the granular phase ($B = 1$). After transition into the granular phase, the stress-strain relationship is governed by $\sigma^b_{ij}$, circumventing the mechanical instability of $\sigma^s_{ij}$ when $\alpha \geq \alpha_{cr}$ (Lyakhovsky & Ben-Zion, 2014).

The mathematical expression of $P(\alpha)$ suggests that the probability of the transition $\approx 0$ when $\alpha \ll \alpha_{cr}$, whereas $P(\alpha) \approx 1$ when $\alpha \gg \alpha_{cr}$. $P(\alpha)$ is proposed according to the Fermi–Dirac distribution (Landau & Lifshitz, 2013) and its extension to the thermodynamics of the granular materials (Edwards, 2005). This expression for the phase transition to granular materials has been validated by McNamara et al. (2009). Particularly for earthquake dynamics, Lyakhovsky et al. (2011) show the solid-granular transition with such expression can reproduce the slip rate time history in analogy to the frictional boundary. With this definition of $P(\alpha)$, the breakage accumulation rate $\dfrac{\partial B}{\partial t}$ in Eq. (1) is very small when the damage variable is well below its critical transition value ($\alpha \ll \alpha_{cr}$).

To fit the governing equations of CDB into the algorithm proposed by Niu et al. (2025) for SeisSol, we summarize Eq. (1) as the following nonlinear hyperbolic system of conservation laws with a source term (Dumbser et al., 2008):

$$\frac{\partial q_p}{\partial t} + \frac{\partial F_p^d(\underline{v}, \underline{\underline{\varepsilon}}, \alpha, B)}{\partial x_d} = s_p(\underline{v}, \underline{\underline{\varepsilon}}, \alpha, B), \tag{3}$$

where $\boldsymbol{q} = (\varepsilon_{xx}, \varepsilon_{yy}, \varepsilon_{zz}, \varepsilon_{xy}, \varepsilon_{yz}, \varepsilon_{zx}, v_x, v_y, v_z, \alpha, B)^T$ is a vector of the conservative variables. $\varepsilon_{xx}$, $\varepsilon_{yy}$, $\varepsilon_{zz}$, $\varepsilon_{xy}$, $\varepsilon_{yz}$, and $\varepsilon_{zx}$ are six components of the strain tenser $\underline{\underline{\varepsilon}} = \varepsilon_{ij}$; $v_x$, $v_y$, and $v_z$ are the three components of the particle velocity vector $\underline{v}$. The flux term $F_p^d$ represents the rates at which the conservative variable $q_p$ gets transferred through a unit area in the direction $x_d$ (LeVeque, 2002). The source vector $s_p = (0, 0, 0, 0, 0, 0, 0, 0, 0, r_\alpha, r_B)^T$ with only two non-zero components $r_\alpha$ and $r_B$ defined in Eq. (2).

We then handle the numerical flux on the frictional interface for dynamic rupture simulation. We first rotate $q_q$ to the face-aligned coordinate system as $q_p^n = T_{rs}^{-1} q_s$, with the rotation matrix $T_{rs}$ given in Niu et al. (2025). For a more accurate estimation of the stress on the fault, we derive the face-aligned conservative variables $q_p^{\sigma,b} = (\sigma_{xx}, \sigma_{yy}, \sigma_{zz}, \sigma_{xy}, \sigma_{yz}, \sigma_{zx}, v_x, v_y, v_z, \alpha, B)^T$ for the stress-velocity form of the wave equations according to Pelties et al. (2012) with the nonlinear stress-strain relationships in Eq. (2). Using $q_p^{\sigma,b}$, we solve the stress on the interface with various types of friction laws (Uphoff, 2020) on the fault interface. We follow the same procedures as described in earlier publications related to SeisSol from Pelties et al. (2012) and refer to them for more detailed descriptions of the formula. As in Eq. (13) of Pelties et al. (2012), the frictional boundary flux is defined with Lamé parameters. We approximate the influence of the damage and breakage variables on the Lamé parameters by keeping the isotropic component of $\sigma_{ij}^s$ and $\sigma_{ij}^b$ in Eq. (2). This approximation leads to the following effective Lamé parameters:

$$\begin{cases} \lambda^{eff} = (1-B)(\lambda_0 - \alpha\gamma_r\epsilon/\sqrt{I_2}) + B(2a_2 + 3a_3\xi + a_1\epsilon/\sqrt{I_2}) \\ \mu^{eff} = (1-B)(\mu_0 - \alpha\xi_0\gamma_r - 0.5\alpha\gamma_r\xi) + B(a_0 + 0.5a_1\xi - 0.5a_3\xi^3) \end{cases}, \quad (4)$$

where $\epsilon = (\varepsilon_{xx} + \varepsilon_{yy} + \varepsilon_{zz})/3$. As shown in Fig. 3 of the main text, the isotropic approximation keeps the numerical stability and still ensures energy conservation throughout the simulations.

## Text S2: Thermodynamic expressions of the continuum damage breakage model

In this section, we summarize the CDBM proposed by Lyakhovsky et al. (2016) to provide a better understanding of the model in terms of its energy balance. The model starts with the first law of thermodynamics,

$$\dot{u} = \underset{=}{\sigma} : \dot{\underset{=}{\varepsilon}} + \dot{q}, \quad (5)$$

where $\dot{(\cdot)}$ denotes the time derivative, $u$ is the specific internal energy of the system normalized by volume, $w$ is the external work per unit volume of the system and $q$ is the absorbed heat from the environment per unit volume of the system. At the time scale of elastodynamic processes, the heat transfer and any possible heat sources are assumed to be negligible, i.e. we assume an adiabatic process where $\dot{q} = 0$. In case of only considering mechanical work, it is $\dot{w} = \underset{=}{\sigma} : \dot{\underset{=}{\varepsilon}} = \sigma_{ij}\dot{\varepsilon}_{ij}$ and $\underset{=}{(\cdot)}$ denotes a tensor of rank two.

The expression of the internal energy depends on the choice of state variables that are used to describe the system. For an elastic material, we chose the strain $\underset{=}{\varepsilon}$ and the specific entropy $s$ as state variables. In addition, to incorporate the damage to the material, we include two more scalar state variables $\alpha$ and $B$. This means $u \equiv u(s, \underset{=}{\varepsilon}, \alpha, B)$.

With the above definitions of state variables, the change of the internal energy in time can be written as

$$\dot{u} = T\dot{s} + \frac{\partial u}{\partial \underline{\underline{\varepsilon}}} : \dot{\underline{\underline{\varepsilon}}} + \frac{\partial u}{\partial \alpha}\dot{\alpha} + \frac{\partial u}{\partial B}\dot{B}, \tag{6}$$

where $T = \dfrac{\partial u}{\partial s} > 0$ is the absolute temperature. If we ignore the coupling between the entropy $s$ and the other state variables, we can define $u = u^s(s) + e(\underline{\underline{\varepsilon}}, \alpha, B)$, where we define $u^s(s)$ as the part of the internal energy that depends only on the entropy $s$, and $e(\underline{\underline{\varepsilon}}, \alpha, B)$ in this work as the mechanical potential energy of rocks.

Different damage models have different ways of defining the internal energy as a function of $\underline{\underline{\varepsilon}}$ and $\alpha$. The combination of Eqs. (5) and (6), together with the previously defined assumptions of $\dot{q} = 0$ and $\dot{w} = \underline{\underline{\sigma}} : \dot{\underline{\underline{\varepsilon}}}$, yield the following results.

$$T\dot{s} = (\underline{\underline{\sigma}} - \frac{\partial e}{\partial \underline{\underline{\varepsilon}}}) : \dot{\underline{\underline{\varepsilon}}} - \frac{\partial e}{\partial \alpha}\dot{\alpha} - \frac{\partial e}{\partial B}\dot{B}. \tag{7}$$

For a spontaneous process in an adiabatic system, $T\dot{s} \geq 0$ for any given $\dot{\varepsilon}$, $\dot{\alpha}$ and $\dot{B}$, which is known as the Clausius–Duhem inequality (Truesdell, 1952). Assuming $\underline{\underline{\sigma}}$ is independent of $\dot{\underline{\underline{\varepsilon}}}$, we derive:

$$\underline{\underline{\sigma}} = \frac{\partial e}{\partial \underline{\underline{\varepsilon}}}. \tag{8}$$

We can then derive the energy dissipation rate of the system from Eqs. (7) and (8),

$$\dot{\mathscr{D}} = T\dot{s} = -\frac{\partial e}{\partial \alpha}\dot{\alpha} - \frac{\partial e}{\partial B}\dot{B}. \tag{9}$$

## Text S3: Energy conservation in continuum damage breakage model and dynamic rupturing

The accumulation of damage in rocks is a thermodynamically irreversible process. This comes with an energy partitioning that is different from the elastic case. The loss of potential energy in the rocks not only transforms into frictional energy on the fault and kinetic energy in the bulk material but dissipates as an entropy increase of the system as well. In this section, we derive the mathematical expression of the dissipated energy and how it is balanced with the change of potential energy, the frictional work on the fault, and the radiated kinetic energy.

We start from the momentum conservation of the system, ignoring the body force, as follows:

$$\rho\frac{\partial v_i}{\partial t} = \frac{\partial \sigma_{ij}}{\partial x_j}. \tag{10}$$

We multiply $v_i$ on both sides of Eq. (10) and integrate it in the entire simulation domain $\Omega$ to derive

$$\int_\Omega v_i\rho\frac{\partial v_i}{\partial t}\mathrm{d}V = \int_\Omega v_i\frac{\partial \sigma_{ij}}{\partial x_j}\mathrm{d}V. \tag{11}$$

We can re-formularize the left-hand-side of Eq. (11) and apply the Gauss theorem on the right-hand-side of Eq. (11). This leads to

$$\int_\Omega \frac{\partial(1/2\rho v_i v_i)}{\partial t}\mathrm{d}V = \int_\Gamma v_i\sigma_{ij}n_j\mathrm{d}S - \int_\Omega \sigma_{ij}\frac{\partial v_i}{\partial x_j}\mathrm{d}V, \tag{12}$$

where $n_j$ is the normal vector of the face element $\Gamma$, $\Gamma = \Gamma^{fault} \cup \Gamma^{surf}$ consists of the fault interfaces $\Gamma^{fault}$ and the boundaries of the entire domain $\Gamma^{surf}$. Since $\sigma_{ij} = \sigma_{ji}$, we

can re-write Eq. (12) as

$$\int_\Omega \frac{\partial(1/2\rho v_i v_i)}{\partial t}\mathrm{d}V = \int_\Gamma v_i\sigma_{ij}n_j\mathrm{d}S - \int_\Omega \sigma_{ij}\frac{1}{2}(\frac{\partial v_i}{\partial x_j} + \frac{\partial v_j}{\partial x_i})\mathrm{d}V. \tag{13}$$

For infinitesimal deformation, the strain tensor $\dot{\varepsilon}_{ij} = \frac{1}{2}(\frac{\partial v_i}{\partial x_j} + \frac{\partial v_j}{\partial x_i})$. We substitute this into Eq. (13) and get

$$\int_\Omega \frac{\partial(1/2\rho v_i v_i)}{\partial t}\mathrm{d}V = \int_\Gamma v_i\sigma_{ij}n_j\mathrm{d}S - \int_\Omega \sigma_{ij}\dot{\varepsilon}_{ij}\mathrm{d}V. \tag{14}$$

From Eqs. (7) and (8), we can derive

$$T\dot{s} + \frac{\partial e}{\partial \alpha}\dot{\alpha} + \frac{\partial e}{\partial B}\dot{B} = 0. \tag{15}$$

If we add Eq. (14) to Eq. (15), substitute the second term on the right-hand-side of Eq. (14) with Eq. (8), and consider the definition of $e$ in Eq. (6), we derive

$$\begin{aligned}\int_\Gamma v_i\sigma_{ij}n_j\mathrm{d}S &= \int_\Omega \frac{\partial(1/2\rho v_i v_i)}{\partial t}\mathrm{d}V + \int_\Omega (\frac{\partial e}{\partial \underline{\underline{\varepsilon}}} : \dot{\underline{\underline{\varepsilon}}} + \frac{\partial e}{\partial \alpha}\dot{\alpha} + \frac{\partial e}{\partial B}\dot{B})\mathrm{d}V + \int_\Omega T\dot{s}\mathrm{d}V \\ &= \int_\Omega \frac{\partial(1/2\rho v_i v_i)}{\partial t}\mathrm{d}V + \int_\Omega \dot{e}\mathrm{d}V + \int_\Omega T\dot{s}\mathrm{d}V.\end{aligned} \tag{16}$$

We define $\dot{W} = \int_{\Gamma^{fault}} v_i\sigma_{ij}n_j\mathrm{d}S$ as the power of frictional force on the fault interfaces, $\dot{W}^s = \int_{\Gamma^{surf}} v_i\sigma_{ij}n_j\mathrm{d}S$ as the power of the external work on the domain boundaries. In our simulations, we set the top surface at $z = 0$ as the free surface and the rest as absorbing boundaries. On the free surface, the traction $\sigma_{ij}n_j = 0$. Our simulation domain is large enough such that the waves do not reach the absorbing boundaries such that $v_i = 0$. Therefore, $W^s$ remains zero in the results shown in Fig. 5 of the main text. We further define $\dot{K} = \int_\Omega \frac{\partial(1/2\rho v_i v_i)}{\partial t}\mathrm{d}V$ as the change rate of kinetic energy, $\dot{E} = \int_\Omega \dot{e}\mathrm{d}V$ as the change rate of mechanical potential energy, and $\dot{\mathcal{D}} = \int_\Omega T\dot{s}\mathrm{d}V$ as the energy dissipation

rate due to the irreversibility of the process. With the above definitions, we derive the following conservation of energy from Eq. (16):

$$\dot{W} = \dot{K} + \dot{E} + \dot{\mathcal{D}} \tag{17}$$

## Text S4: Comparison of off-faut shear band angles between analytical and numerical simulations

The theory of CDB describes the internal friction angle of the material in analogy to Byerlee (1978). The equivalent internal friction angle in the CDB model is determined from the nonlinear material properties $\xi_0$ in Eq. (2). As listed in Table S1, $\xi_0$ is -0.75 (Lyakhovsky et al., 1997). This corresponds to an internal friction angle of 43 degrees. In the simulation of Fig. 3f, the angle between the maximum compressive principal stress and the fault plane is 59.1 degrees. The two conjugate weak planes should take an angle of 45 - 43/2 = 23.5 degrees from the maximum compressive principal stress. This corresponds to angles of 59.1 - 23.5 = 35.6 degrees or 59.1 + 23.5 = 82.6 degrees between the weak plane and the fault plane. We find the theoretical angle of 35.6 degrees from the fault plane in Fig. 3f (red dashed line) agrees with our numerical simulation results. The same angles are kept as the depth changes from 7.5 to 2.5 km in Fig. 3d and Fig. 3e. We further verify the consistency by varying the angle between the maximum compressive principal stress and the fault plane from 59.1 degrees to 54.6 degrees in Fig. 3c. This time, the weak plane from numerical simulation also takes a smaller angle from the fault plane, which is around 31.1 degrees. The damage pattern is also stable when refining mesh sizes from 100 m to 25 m. We show the mesh-independency in Fig. S1.

## Text S5: Limitations on high-order polynomials in DG elements for localized damage

Highly localized damage creates non-smooth distributions of the breakage variable within some elements, especially challenging for shape functions with polynom ial degrees $p > 1$. Such shape functions introduce significant intra-element heterogeneity (Dumbser et al., 2007; Dumbser & Loubère, 2016), amplifying non-smoothness and potentially leading to physically unrealistic values of damage ($\alpha$) and breakage ($B$) variables. Our simulations show that employing linear Dubiner's basis functions ($p = 1$) effectively mitigates these issues (Cockburn et al., 2012; Wollherr et al., 2018). For higher-order polynomial functions ($p \geq 2$), alternative strategies such as artificial viscosity (Hartmann & Houston, 2002), filtering methods (Radice & Rezzolla, 2011), or WENO-based reconstructions (Qiu & Shu, 2004) may be necessary to maintain smoothness and physical realism. In addition, oscillatory regions can be identified, allowing the introduction of element-local smoothing (Diot et al., 2013; Loubere et al., 2014).

The solid-granular phase transition inside the damage zone also contributes to secondary waves and high-frequency radiation. We show in Fig. S2 how the high frequency depends on the mesh. Compared to the elastic case (the dashed black curve), the off-fault phase transition generates more energy beyond 0.4 Hz on all three mesh resolutions. The shape of the power spectral density keeps a similar amplitude up to around 5 Hz. Beyond this frequency, a finer mesh resolves a greater energy.

## Text S6: Supershear transition and cohesive zone width with off-fault damage

In this section, we address the impacts of off-fault damage processes on two important aspects of the dynamic rupture: (1) supershear transition and (2) cohesive zone size.

A rupture front that propagates at an intersonic speed (supershear) can significantly change the directivity of earthquakes. In supershear, the constructive interference of the waves radiated from a Mach front results in much stronger ground motions than a wave front that is transported at sub-Rayleigh speeds (Bernard & Baumont, 2005; Dunham & Archuleta, 2005; Bhat et al., 2007). The supershear transition in this work in Section 3.1 results from the daughter crack that nucleates in front of the sub-Rayleigh rupture due to the local dynamic stress peak (Andrews, 1976; Dunham, 2007). We show in Fig. S3b how the damage coefficient $C_d$ influences the variation of supershear transition with the strength excess to stress drop ratio $S$ defined as

$$S = \frac{\sigma_0 \mu_s - \tau_0}{\tau_0 - \sigma_0 \mu_d}, \tag{18}$$

where $\sigma_0$ and $\tau_0$ are the initial normal and shear traction on the fault, $\mu_s$ and $\mu_d$ are the static and dynamic friction coefficiein in the linear slip-weakening law.

We here define that the supershear transition begins from the point where the peak slip rate reaches a local maximum, as marked with the two dash-dotted arrows in Fig. S3a according to Gabriel et al. (2012). The red line in Fig. S3a marks the $r_{crit}$ where we nucleate the dynamic rupture (Harris et al., 2018).

The cohesive zone (also known as the breakdown or process zone) is defined as the area behind the rupture front where the shear stress drops from its static value to its dynamic value (Day et al., 2005). Within the cohesive zone, the slip rate and the fault traction change significantly. This makes the dimension of the cohesive zone an important length

scale to resolve in mesh refinement. We show in Fig. S4 how the cohesive zone is altered by the off-fault damage.

**Text S7: Evolution of traction and slip rate on the two faults in TPV23**

We use this section to provide the slip rate and shear traction distribution on the two faults in the step-over set up in Section 3.3 at different times after the nucleation of the dynamic rupture on the first fault. We show in Fig. S5a-1 to S5a-4 the distribution of slip rate on the two faults at 4s, 7s, 35 s and 40 s, and in Fig. S5b-1 to S5b-4 the distribution of shear traction on the two faults at 4s, 7s, 35 s and 40 s.

**Movie S1.** The left column shows the evolution of rupture speed, shear modulus reduction, and strain ratio $\xi$ from 0.0 to 3.0 s after the rupture onset in Fig. 1 of the main text. The right column shows the depth-dependent off-fault damage zone and how it evolves in time.

**Movie S2.** The left and right panels show the evolution of the cross-fault distribution of, respectively, the localized shear bands and the magnitude of the velocity vector from 0.0 to 4.0 s after the rupture onset at the 7.5 km depth in Fig. 3 of the main text.

**Movie S3.** The top left, top right, and bottom right panels show the evolution of shear modulus reduction, shear traction, and slip rate from 0.0 to 55.0 s after the rupture onset on F1 in Fig. 6 of the main text. The bottom left panel shows how the localized modulus reduction zone extends from F1 to F2.

**Movie S4.** Comparison, between the elastic (left panels) and the CDB model (right panels), of the evolution of shear traction (top panels) and slip rate (bottom panels) from 0.0 to 55.0 s after the rupture onset on F1 in Fig. 6 of the main text.

## References

Andrews, D. (1976). Rupture velocity of plane strain shear cracks. *Journal of Geophysical Research*, *81*(32), 5679–5687.

Bernard, P., & Baumont, D. (2005). Shear mach wave characterization for kinematic fault rupture models with constant supershear rupture velocity. *Geophysical Journal International*, *162*(2), 431–447.

Bhat, H. S., Dmowska, R., King, G. C., Klinger, Y., & Rice, J. R. (2007). Off-fault damage patterns due to supershear ruptures with application to the 2001 $M_W$ 8.1 Kokoxili (Kunlun) Tibet earthquake. *Journal of Geophysical Research: Solid Earth*, *112*(B6).

Byerlee, J. (1978). Friction of rocks. *Rock friction and earthquake prediction*, 615–626.

Cockburn, B., Karniadakis, G. E., & Shu, C.-W. (2012). *Discontinuous galerkin methods: theory, computation and applications* (Vol. 11). Springer Science & Business Media.

Day, S. M., Dalguer, L. A., Lapusta, N., & Liu, Y. (2005). Comparison of finite difference and boundary integral solutions to three-dimensional spontaneous rupture. *Journal of Geophysical Research: Solid Earth*, *110*(B12).

Diot, S., Loubère, R., & Clain, S. (2013). The multidimensional optimal order detection method in the three-dimensional case: very high-order finite volume method for hyperbolic systems. *International Journal for Numerical Methods in Fluids*, *73*(4), 362–392.

Dumbser, M., Balsara, D. S., Toro, E. F., & Munz, C.-D. (2008). A unified framework for the construction of one-step finite volume and discontinuous Galerkin schemes on unstructured meshes. *Journal of Computational Physics*, *227*(18), 8209–8253.

Dumbser, M., Käser, M., & Toro, E. F. (2007). An arbitrary high-order discontinuous galerkin method for elastic waves on unstructured meshes-v. local time stepping and

p-adaptivity. *Geophysical Journal International*, *171*(2), 695–717.

Dumbser, M., & Loubère, R. (2016). A simple robust and accurate a posteriori sub-cell finite volume limiter for the discontinuous galerkin method on unstructured meshes. *Journal of Computational Physics*, *319*, 163–199.

Dunham, E. M. (2007). Conditions governing the occurrence of supershear ruptures under slip-weakening friction. *Journal of Geophysical Research: Solid Earth*, *112*(B7).

Dunham, E. M., & Archuleta, R. J. (2005). Near-source ground motion from steady state dynamic rupture pulses. *Geophysical Research Letters*, *32*(3).

Edwards, S. (2005). The full canonical ensemble of a granular system. *Physica A: Statistical Mechanics and its Applications*, *353*, 114–118.

Einav, I. (2007a). Breakage mechanics—part ii: Modelling granular materials. *Journal of the Mechanics and Physics of Solids*, *55*(6), 1298–1320.

Einav, I. (2007b). Breakage mechanics—part i: theory. *Journal of the Mechanics and Physics of Solids*, *55*(6), 1274–1297.

Gabriel, A.-A., Ampuero, J.-P., Dalguer, L., & Mai, P. M. (2012). The transition of dynamic rupture styles in elastic media under velocity-weakening friction. *Journal of Geophysical Research: Solid Earth*, *117*(B9).

Harris, R. A., Barall, M., Aagaard, B., Ma, S., Roten, D., Olsen, K., ... Dalguer, L. (2018). A suite of exercises for verifying dynamic earthquake rupture codes. *Seismological Research Letters*, *89*(3), 1146-1162.

Hartmann, R., & Houston, P. (2002). Adaptive discontinuous Galerkin finite element methods for the compressible Euler equations. *Journal of Computational Physics*, *183*(2), 508–532.

Landau, L. D., & Lifshitz, E. M. (2013). *Course of theoretical physics.* Elsevier.

LeVeque, R. J. (2002). *Finite volume methods for hyperbolic problems* (Vol. 31). Cambridge university press.

Loubere, R., Dumbser, M., & Diot, S. (2014). A new family of high order unstructured mood and ader finite volume schemes for multidimensional systems of hyperbolic conservation laws. *Communications in Computational Physics*, *16*(3), 718–763.

Lyakhovsky, V., & Ben-Zion, Y. (2014). A continuum damage–breakage faulting model and solid-granular transitions. *Pure and Applied Geophysics*, *171*, 3099–3123.

Lyakhovsky, V., Ben-Zion, Y., & Agnon, A. (1997). Distributed damage, faulting, and friction. *Journal of Geophysical Research: Solid Earth*, *102*(B12), 27635–27649.

Lyakhovsky, V., Ben-Zion, Y., Ilchev, A., & Mendecki, A. (2016). Dynamic rupture in a damage-breakage rheology model. *Geophysical Journal International*, *206*(2), 1126–1143.

Lyakhovsky, V., Hamiel, Y., & Ben-Zion, Y. (2011). A non-local visco-elastic damage model and dynamic fracturing. *Journal of the Mechanics and Physics of Solids*, *59*(9), 1752–1776.

McNamara, S., Richard, P., De Richter, S. K., Le Caër, G., & Delannay, R. (2009). Measurement of granular entropy. *Physical Review E—Statistical, Nonlinear, and Soft Matter Physics*, *80*(3), 031301.

Niu, Z., Gabriel, A.-A., Wolf, S., Ulrich, T., Lyakhovsky, V., & Igel, H. (2025). *A discontinuous galerkin method for simulating 3d seismic wave propagation in nonlinear rock models: Verification and application to the 2015 mw 7.8 gorkha earthquake.* Retrieved from `https://arxiv.org/abs/2502.09714`

Pelties, C., De la Puente, J., Ampuero, J.-P., Brietzke, G. B., & Käser, M. (2012). Three-dimensional dynamic rupture simulation with a high-order discontinuous Galerkin method on unstructured tetrahedral meshes. *Journal of Geophysical Research: Solid Earth*, *117*(B2).

Qiu, J., & Shu, C.-W. (2004). Hermite WENO schemes and their application as limiters for Runge–Kutta discontinuous Galerkin method: one-dimensional case. *Journal of Computational Physics*, *193*(1), 115–135.

Radice, D., & Rezzolla, L. (2011). Discontinuous Galerkin methods for general-relativistic hydrodynamics: Formulation and application to spherically symmetric spacetimes. *Physical Review D*, *84*(2), 024010.

Truesdell, C. (1952). The mechanical foundations of elasticity and fluid dynamics. *Journal of Rational Mechanics and Analysis*, *1*, 125–300.

Uphoff, C. (2020). *Flexible model extension and optimisation for earthquake simulations at extreme scales* (Unpublished doctoral dissertation). Technische Universität München.

Wollherr, S., Gabriel, A.-A., & Uphoff, C. (2018). Off-fault plasticity in three-dimensional dynamic rupture simulations using a modal Discontinuous Galerkin method on unstructured meshes: implementation, verification and application. *Geophysical Journal International*, *214*(3), 1556–1584.

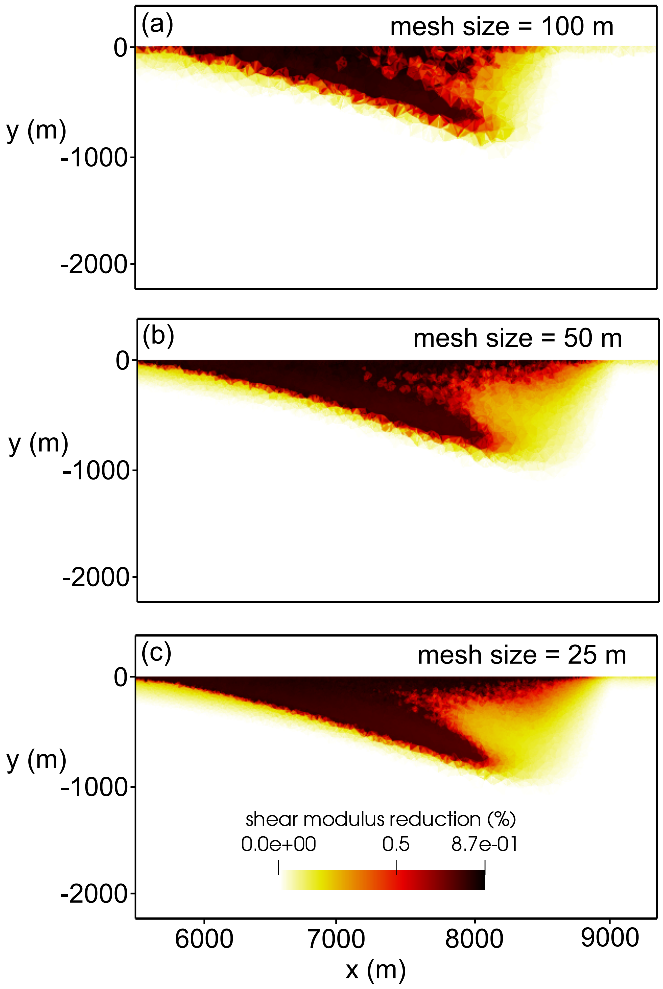


Figure S1: The spatial distribution of the localized shear modulus reduction, zoomed in on the region within the dashed red rectangle in Fig. 3b. The largest tetrahedral element size in (a), (b) and (c) are, respectively, 100 m, 50 m and 25 m.

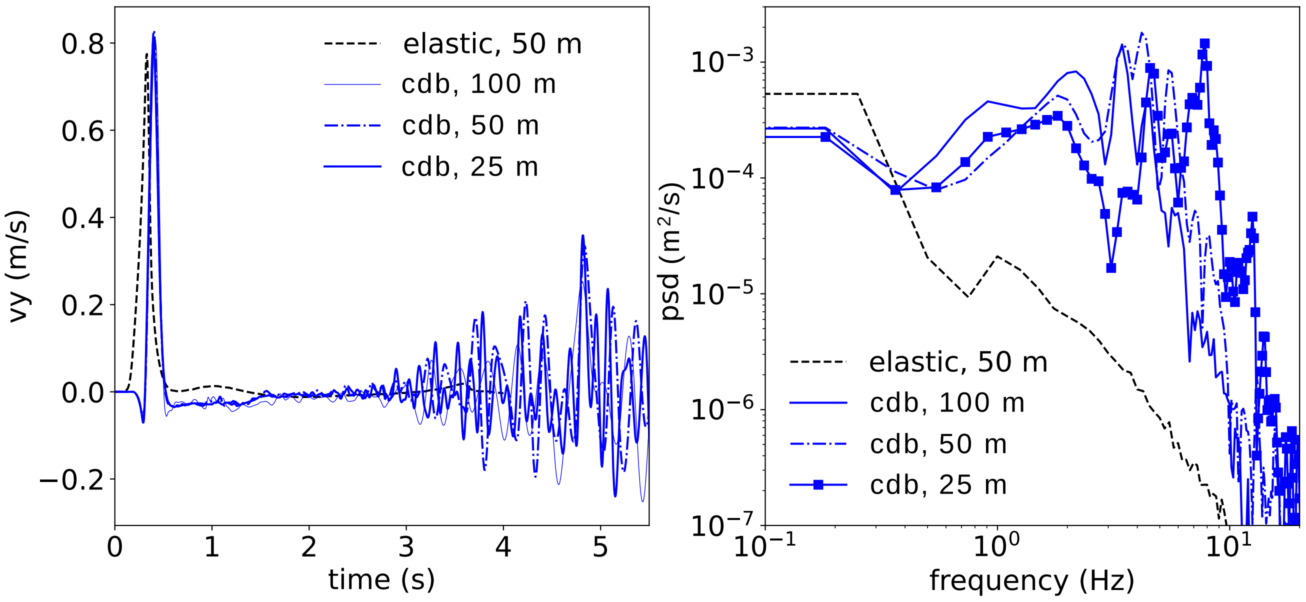


Figure S2: (a) Particle velocity along $y$-axis recorded at the red rectangle in Fig. 3c in the main text. The dashed black curve shows the reference solution when the off-fault material is purely elastic, with a mesh refinement up to 50 m next to the fault plane. We show side-by-side the recorded time series when the off-fault damage in the CDB model is considered with a mesh refinement up to 100 m (the thin solid blue curve), 50 m (the dashed blue curve) and 25 m (the thick solid blue curve). (b) The power spectral density (psd) of the particle velocity along $y$-axis transformed from the corresponding time series in (a).

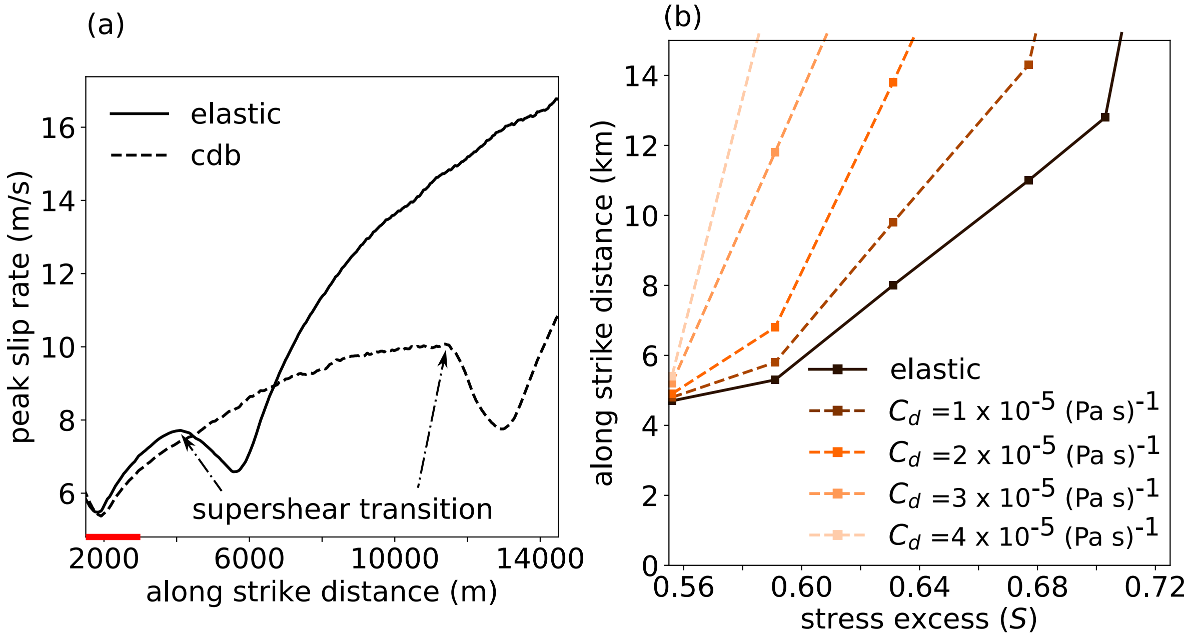


Figure S3: Variation in the point of supershear transition during the fault rupturing. (a) Changes of peak slip rate in the along strike for both elastic (the solid curve) and CDB (the dashed curve) off-fault material models. The two dash-dotted arrows mark the location where we define as the point of supershear transition. The red line marks region where we nucleate the dynamic rupture (Harris et al., 2018). (b) Variation in the point of supershear transition in the along strike direction with stress excess $S$. The solid black curve show the variation in elastic case; while the color-coded curves in orange show the variation in CDB model case, with $C_d = 1 \times 10^{-5}$, $2 \times 10^{-5}$, $3 \times 10^{-5}$ and $4 \times 10^{-5}$ (Pa·s)$^{-1}$. The rest of the parameters are the same as listed in Table S1.

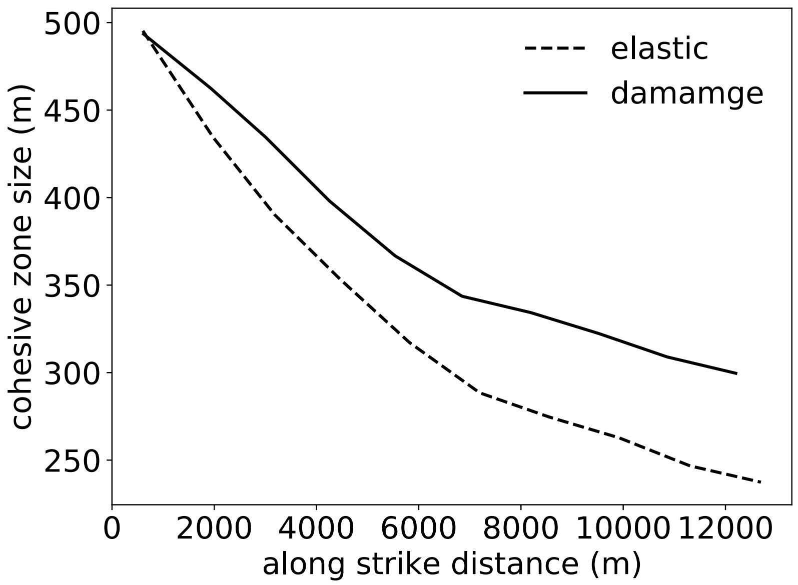


Figure S4: Variation of the cohesive zone width in the along strike direction for both elastic (the dashed curve) and CDB (the solid curve) model case. In the CDB model case, $C_d = 3 \times 10^{-5}$ (Pa·s)$^{-1}$ with the rest of the parameters same as those in Table S1.

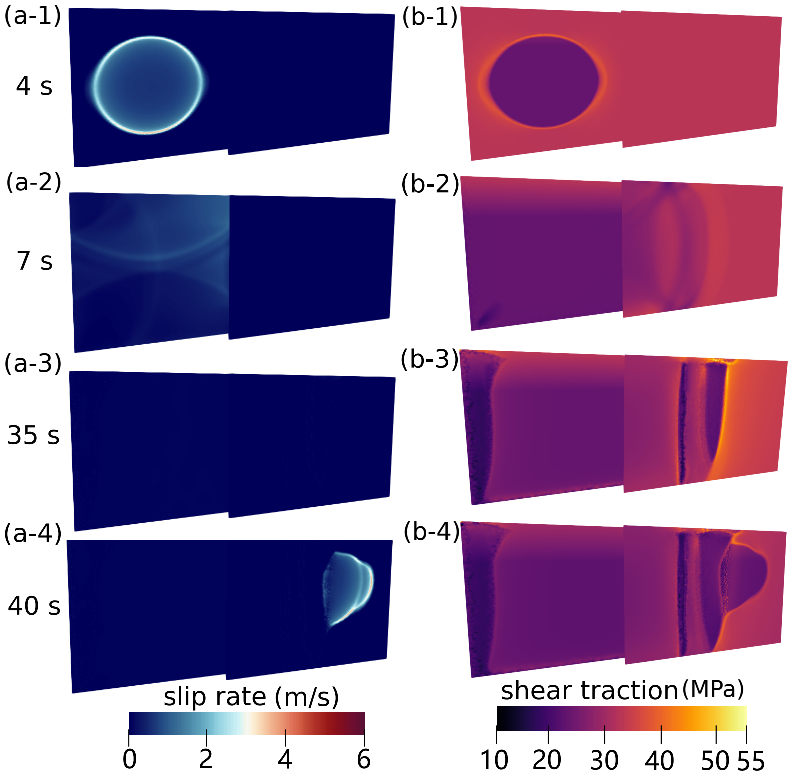


Figure S5: Slip rate (a-1 to a-4) and shear traction (b-1 to b-4) distribution on the two fault planes at 4, 7, 35, and 40 s for the step-over setup in Fig. 6 in the main text.

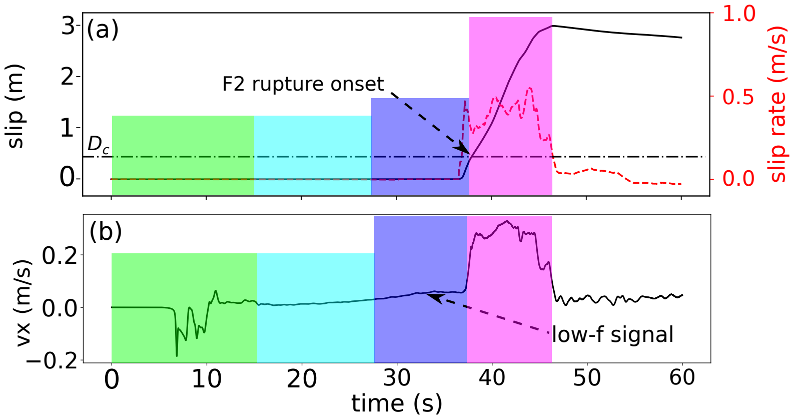


Figure S6: Supplementary results for the delayed dynamic triggering across fault segments due to off-fault damage in Fig. 6. (a) On-fault slip (the solid black curve) and slip rate (the dashed red curve) at the receiver location indicated in Fig. 6b. The dash-dotted black curve marks the critical slip distance $D_c = 0.4$ in the linear slip weakening law. The dashed black arrow marks the onset of spontaneous rupture on fault F2. (b) Off-fault $x$-component of the velocity field ($v_x$) at (12.5, -2.9, -7.5) km, which is next to the location of the on-fault receiver indicated with the cyan rectangle in Fig. 6b.

Table S1: Summary of model parameters for tpv3. The nonlinear modulus $\gamma_r$ and the granular phase moduli from $a_0$ to $a_3$ are computed according to Lyakhovsky & Ben-Zion (2014), with a strain invariants ratio for onset of breakage decrease $\xi_d$ = -0.9 defined therein. The stress component pair $(\sigma_{xx}, \sigma_{zz})$ = (-71, -71) MPa and (-45, -118) MPa correspond to the maximum compressive stress oriented, respectively, 59.1 and 54.6 degrees from $x$-axis.

| | Parameters | Values | Units | Parameters | Values | Units |
|---|---|---|---|---|---|---|
| fault | $\sigma_{xx}$ | -71, -45 | MPa | $D_c$ | 0.3 | m |
| | $\sigma_{yy}$ | -120 | MPa | $\mu_s$ | 0.667 | 1 |
| | $\sigma_{zz}$ | -71, -118 | MPa | $\mu_d$ | 0.425 | 1 |
| | $\sigma_{xy}$ | 70 | MPa | $\sigma_{yz}$, $\sigma_{zx}$ | 0 | MPa |
| bulk material | $\lambda_0$ | 32 | GPa | $a_0$ | 8.42 | GPa |
| | $\mu_0$ | 32 | GPa | $a_1$ | $-23.79$ | GPa |
| | $\gamma_r$ | 37.2 | GPa | $a_2$ | 20.90 | GPa |
| | $\xi_0$ | -0.75 | 1 | $a_3$ | -5.39 | GPa |
| | $C_d$ | $6.0 \times 10^{-5}$ | $(\text{Pa·s})^{-1}$ | $C_B$ | $100C_d$ | $(\text{Pa·s})^{-1}$ |
| | $\beta_{cr}$ | 0.05 | 1 | $\rho$ | 2760 | kg/m$^3$ |

Table S2: Summary of model parameters for tpv23. The nonlinear modulus $\gamma_r$ and the granular phase moduli from $a_0$ to $a_3$ are computed according to Lyakhovsky & Ben-Zion (2014), with a strain invariants ratio for onset of breakage decrease $\xi_d = -0.9$ defined therein.

| | Parameters | Values | Units | Parameters | Values | Units |
|---|---|---|---|---|---|---|
| fault | $\sigma_{xx}$ | -25 | MPa | $D_c$ | 0.3 | m |
| | $\sigma_{yy}$ | -60 | MPa | $\mu_s$ | 0.548 | 1 |
| | $\sigma_{zz}$ | -25 | MPa | $\mu_d$ | 0.373 | 1 |
| | $\sigma_{xy}$ | 29.38 | MPa | $\sigma_{yz}$, $\sigma_{zx}$ | 0 | MPa |
| bulk material | $\lambda_0$ | 32 | GPa | $a_0$ | 8.42 | GPa |
| | $\mu_0$ | 32 | GPa | $a_1$ | -23.79 | GPa |
| | $\gamma_r$ | 37.2 | GPa | $a_2$ | 20.90 | GPa |
| | $\xi_0$ | -0.75 | 1 | $a_3$ | -5.39 | GPa |
| | $C_d$ | $5.0 \times 10^{-6}$ | $(\text{Pa·s})^{-1}$ | $C_B$ | $100C_d$ | $(\text{Pa·s})^{-1}$ |
| | $\beta_{cr}$ | 0.05 | 1 | $\rho$ | 2760 | kg/m$^3$ |
